# Supplementary material for: TSoR: TCP Socket over RDMA Container Network for Cloud Native Computing
Source: arXiv:2305.10621 source file (2023-05-18)
Supplement: Supplementary file 1 [file supplement.tex]

\newpage
% \tableofcontents
